# Supplementary material for: Correlated Electronic Properties of Some Graphene Nanoribbons: A DMRG Study
Source: arXiv:1601.02398 ancillary file (2016-07-18)
Supplement: Supplementary file 1 [file supplemental.pdf]

# Supplemental Material: Correlated Electronic Properties of Some Graphene Nanoribbons: A DMRG Study

V. M. L. Durga Prasad Goli,* Suryoday Prodhan,† and S. Ramasesha‡

*Solid State and Structural Chemistry Unit,*

*Indian Institute of Science, Bangalore-560012, India.*

Sumit Mazumdar§

*Department of Physics, University of Arizona, Tucson, Arizona 85721, USA. and*

*College of Optical Sciences, University of Arizona, Tucson, Arizona 85721, USA.*

* Electronic mail:durgaprasad.vml@gmail.com

† Electronic mail: suryodayp@sscu.iisc.ernet.in

‡ Electronic mail: ramasesh@sscu.iisc.ernet.in

§ Electronic mail: sumit@physics.arizona.edu

The contents of this supplemental material are:

1. Construction scheme of 6-AGNR and 5-AGNR in the infinite DMRG method.

2. Full DMRG sweep scheme of 16-site 6-AGNR in the finite DMRG method.

3. Full DMRG sweep scheme of 20-site 5-AGNR in the finite DMRG method.

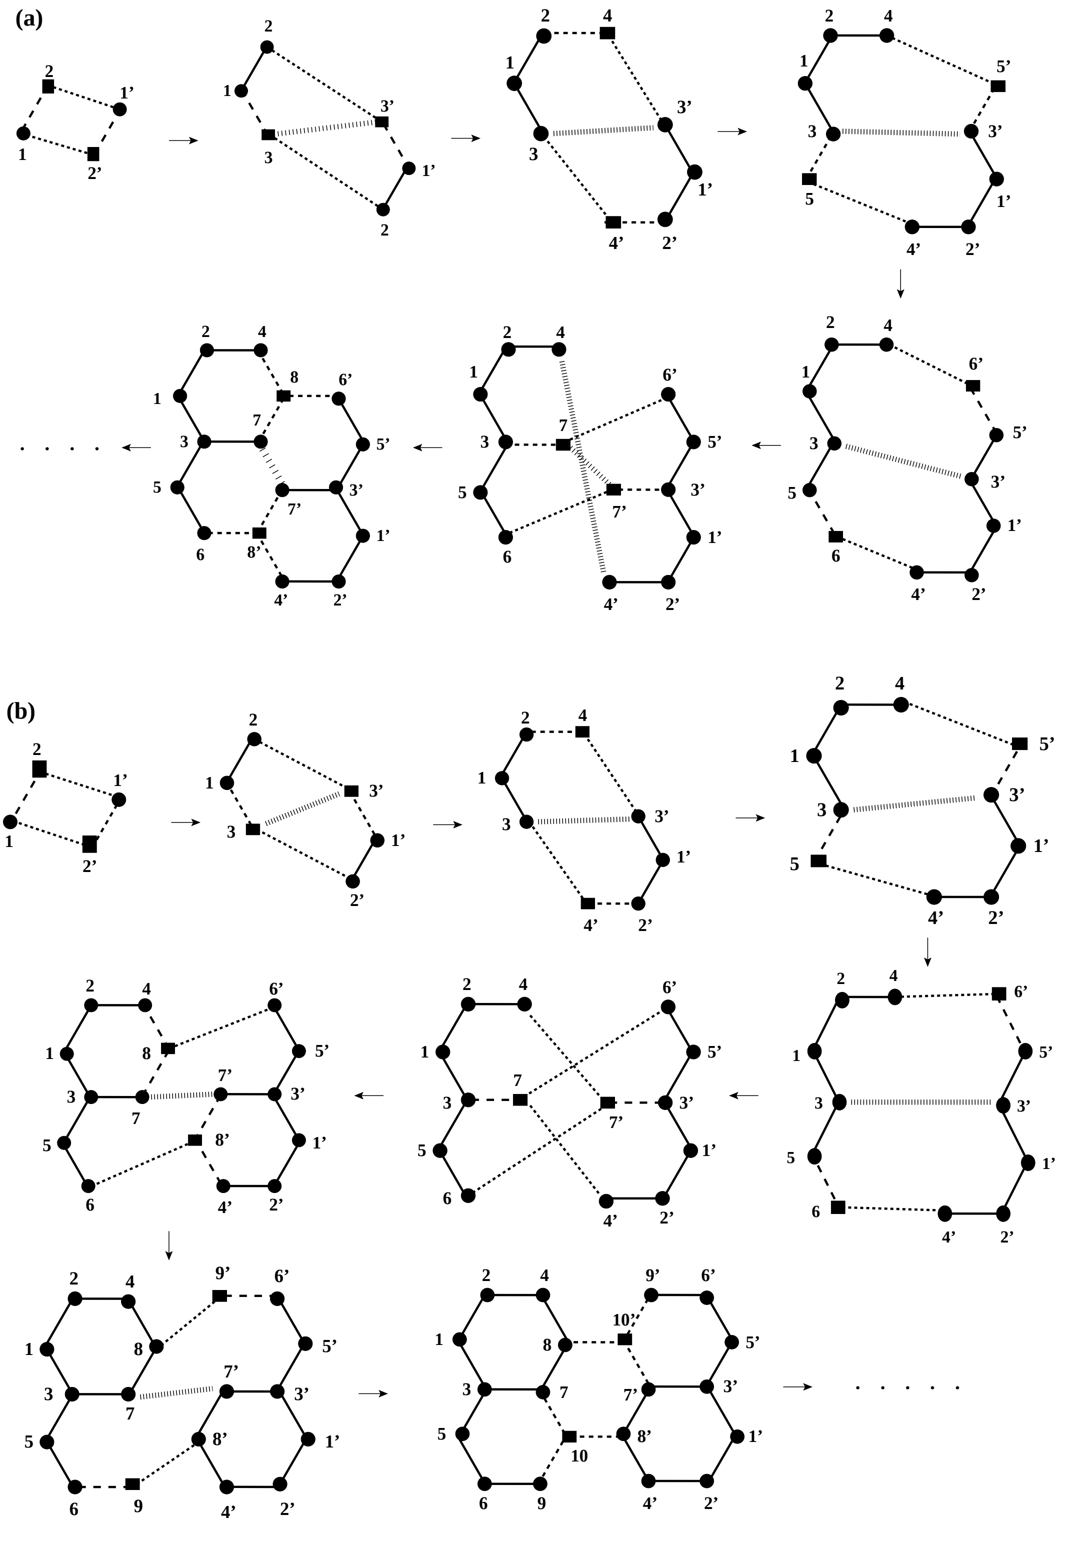


FIG. 1. Construction scheme of (a) 6-AGNR and (b) 5-AGNR in the infinite DMRG method. All symbols are defined in the caption of Fig. 2 in the main manuscript

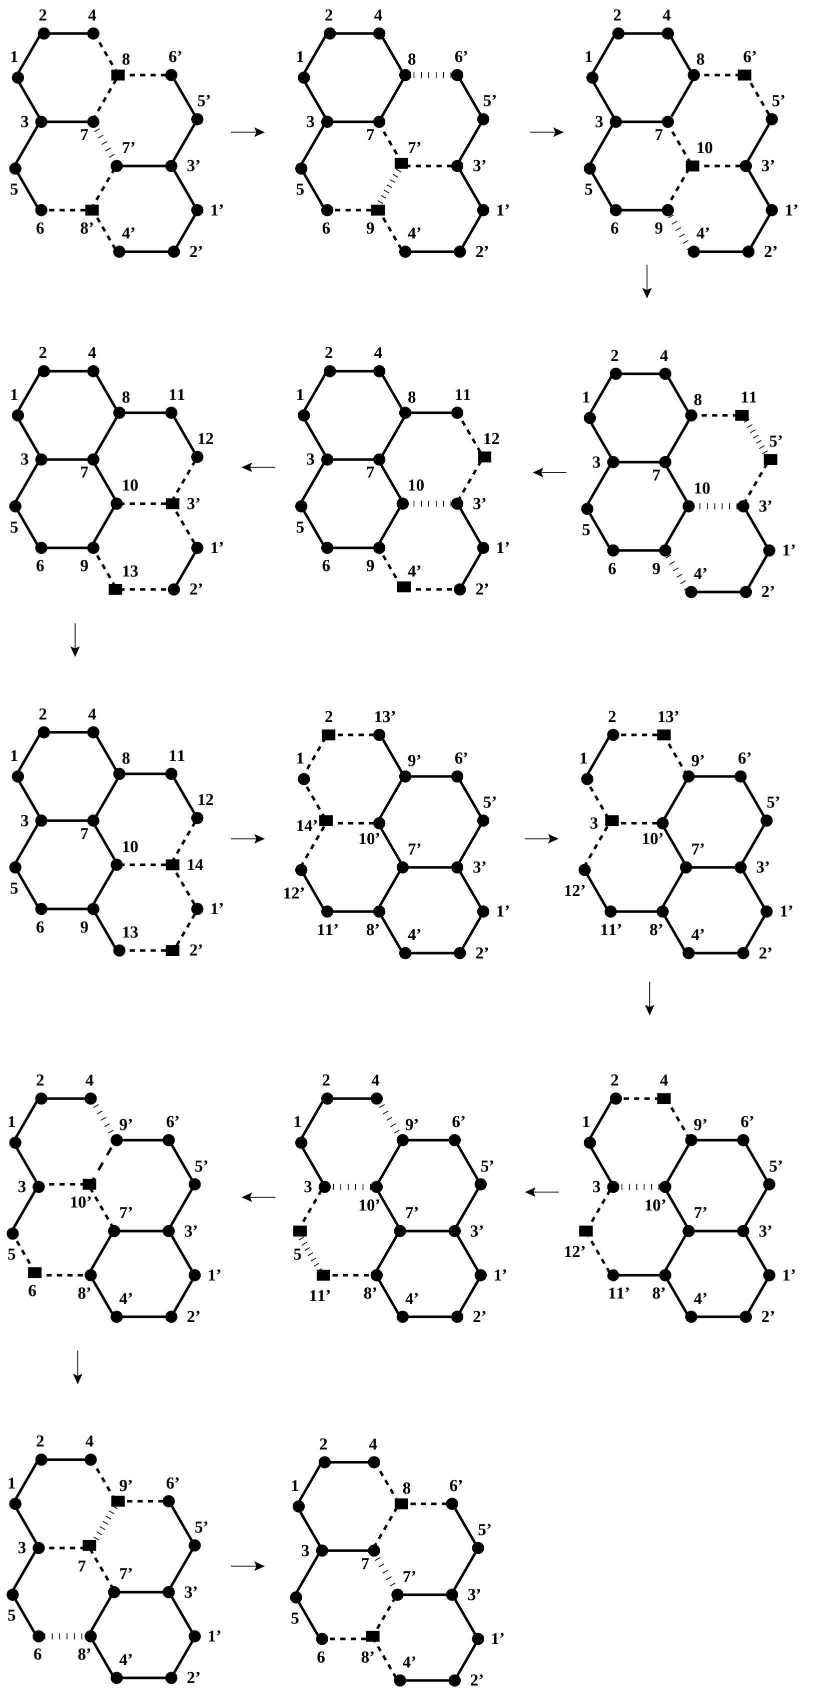

FIG. 2. Full DMRG sweep scheme of 16-site 6-AGNR in the finite DMRG method.

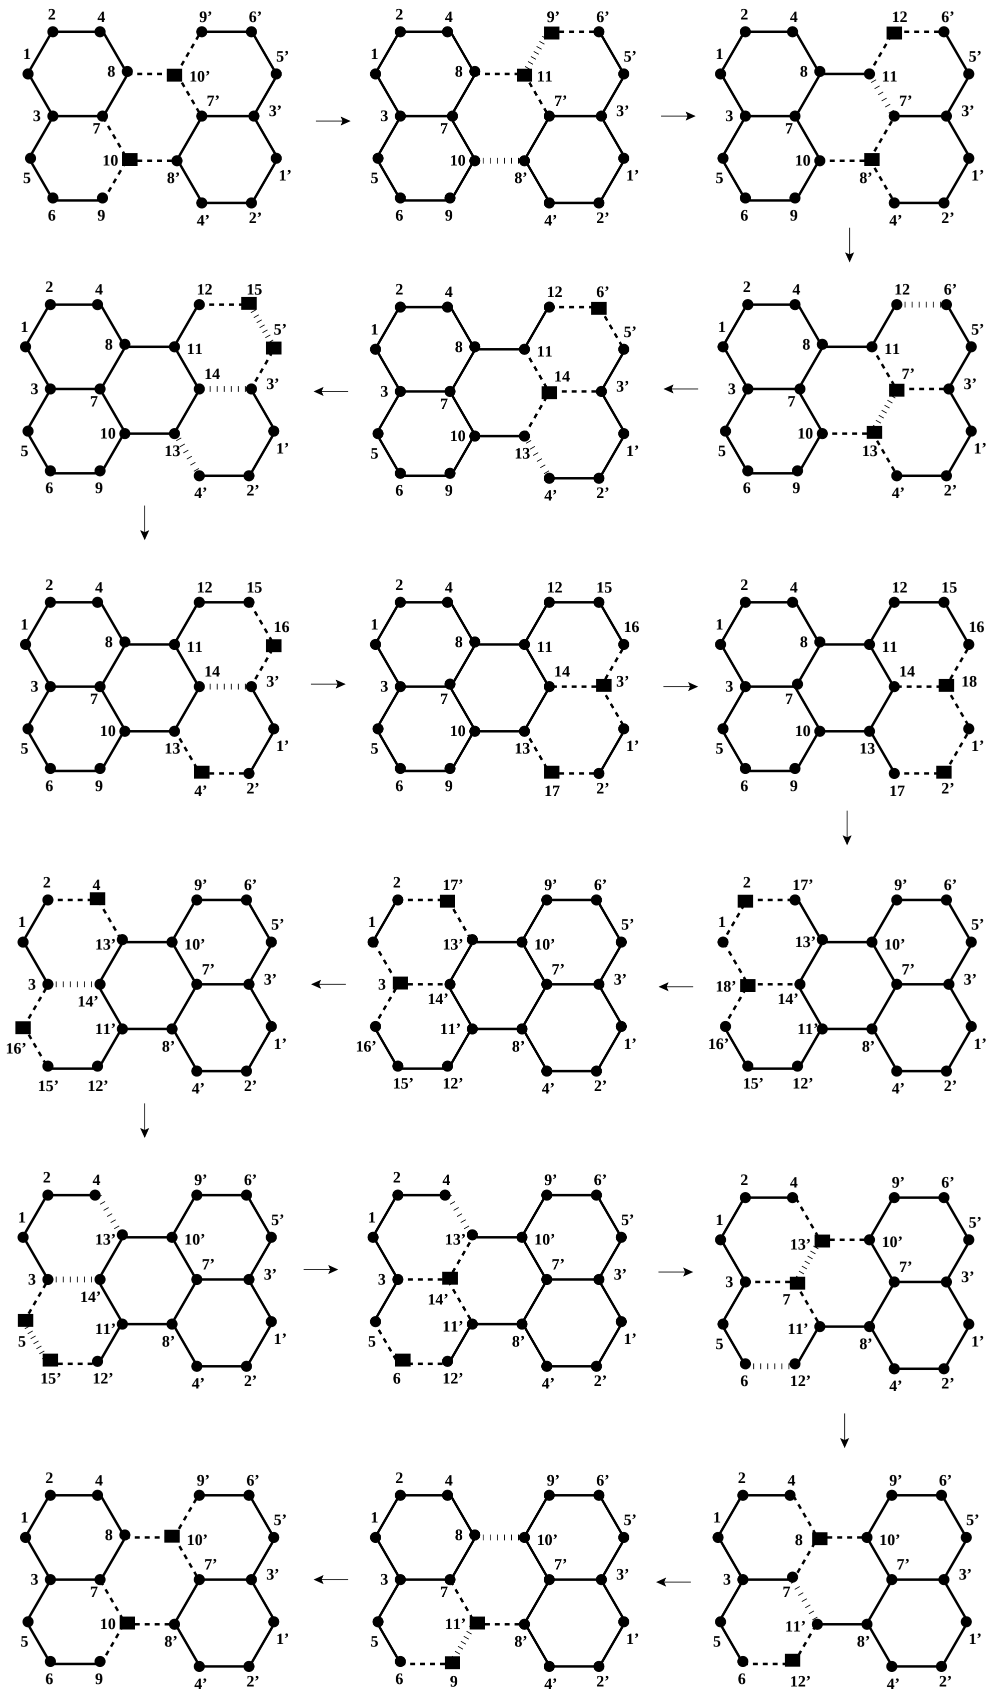

FIG. 3. Full DMRG sweep scheme of 20-site 5-AGNR in the finite DMRG method.
